# Supplementary material for: Natural orbitals and sparsity of quantum mutual information
Source: arXiv:2308.08056 source file (2023-08-15)
Supplement: Supplementary file 1 [file supplementary.tex]

\documentclass[10pt]{extarticle}
\usepackage[margin=0.9 in]{geometry}
\usepackage{amsmath}
\usepackage{amsfonts}
\usepackage{amssymb}
\usepackage{graphicx}
\usepackage{grffile}
\usepackage{braket}
\usepackage{bbold}
\usepackage{subcaption}
\usepackage{stfloats}

\usepackage{listings}
\usepackage{bm}
\usepackage{qcircuit}
\usepackage{xcolor}

\pdfsuppresswarningpagegroup=1

\title{Supplementary Material}

\author{Leonardo Ratini, Chiara Capecci and Leonardo Guidoni}

\begin{document}
\maketitle
\section{Supplemental Material: quantum mutual information}
Below are reported the quantum mutual information maps for the other molecules considered in this work. For each figure, we have the VQE state (a), the WAHTOR state (b) and the ground state (c,d,e). The first one is expressed in the HF basis, the second one in the converged molecular basis and the third one in three different basis sets: HF, converged and natural orbitals set. 
%For each molecule, we note that the quantum mutual information in the WAHTOR state is distributed on the qubit pairs as well as in the ground state expressed in the natural orbital basis. As more the converged state is similar to the ground state as more the quantum mutual information maps are similar.

\begin{figure*}[!htb]
\centering
\subfloat[VQE state in HF canonical orbitals]
   {\includegraphics[width=0.45\textwidth]{grafici/supplementary/H2/VQE in initial basis.png}} \quad
\subfloat[WAHTOR state in WAHTOR-optimized orbitals]
   {\includegraphics[width=0.45\textwidth]{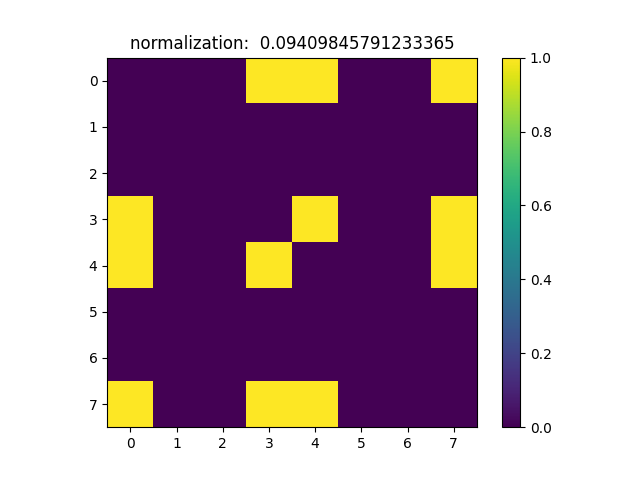}} \\
\subfloat[Groundstate in HF canonical orbitals]
   {\includegraphics[width=0.45\textwidth]{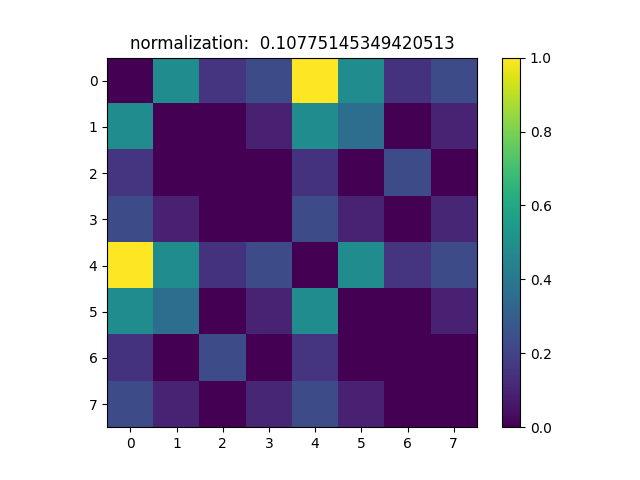}} \quad
\subfloat[Groundstate in WAHTOR-optimized orbitals]
   {\includegraphics[width=0.45\textwidth]{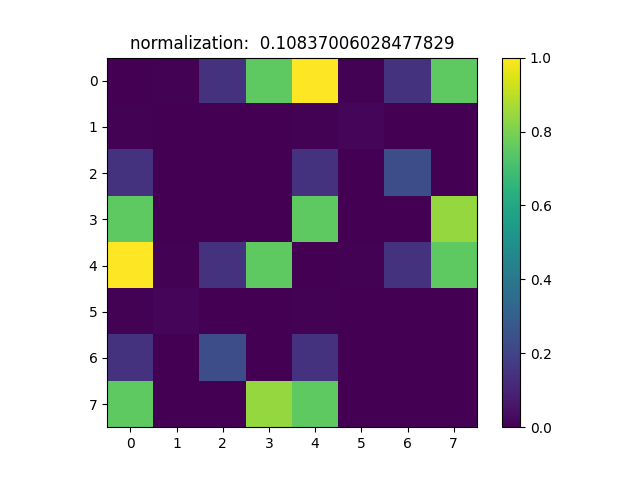}} \quad   
\subfloat[Groundstate in natural orbitals]
   {\includegraphics[width=0.45\textwidth]{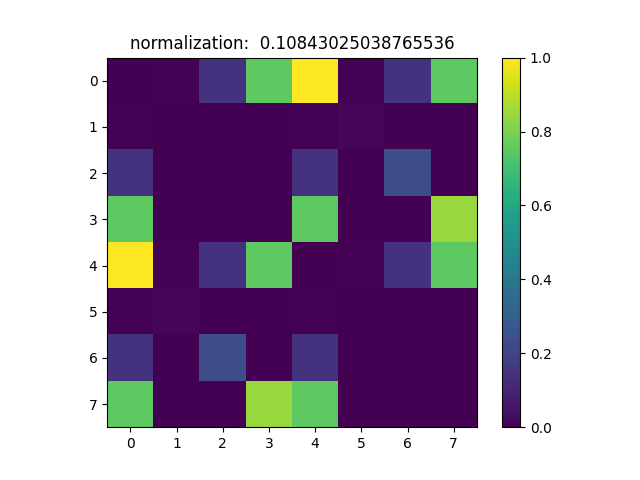}} \\
\caption{Quantum mutual information for $H_2$ molecule.}
\label{fig:H2}
\end{figure*}

\begin{figure*}[!htb]
\centering
\subfloat[VQE state in HF canonical orbitals]
   {\includegraphics[width=0.45\textwidth]{grafici/supplementary/LiH/VQE in initial basis.png}} \quad
\subfloat[WAHTOR state in WAHTOR-optimized orbitals]
   {\includegraphics[width=0.45\textwidth]{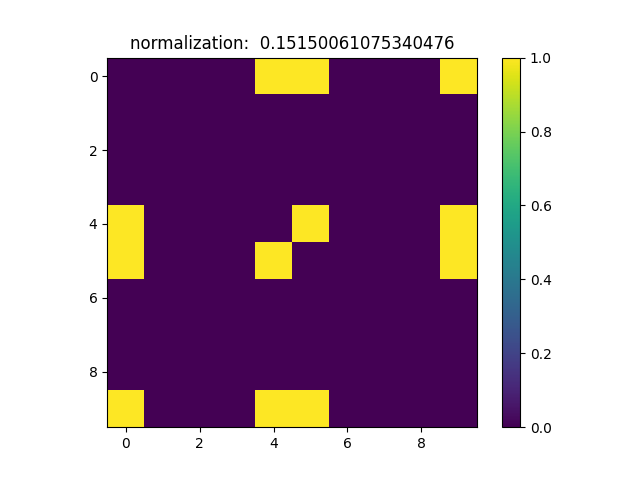}} \\
\subfloat[Groundstate in HF canonical orbitals]
   {\includegraphics[width=0.45\textwidth]{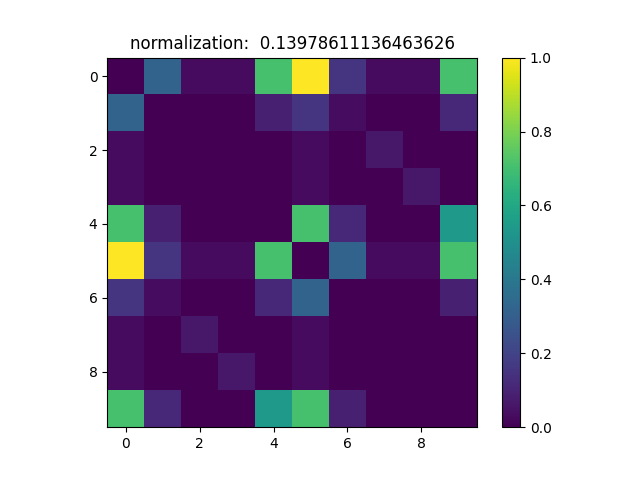}} \quad
\subfloat[Groundstate in WAHTOR-optimized orbitals]
   {\includegraphics[width=0.45\textwidth]{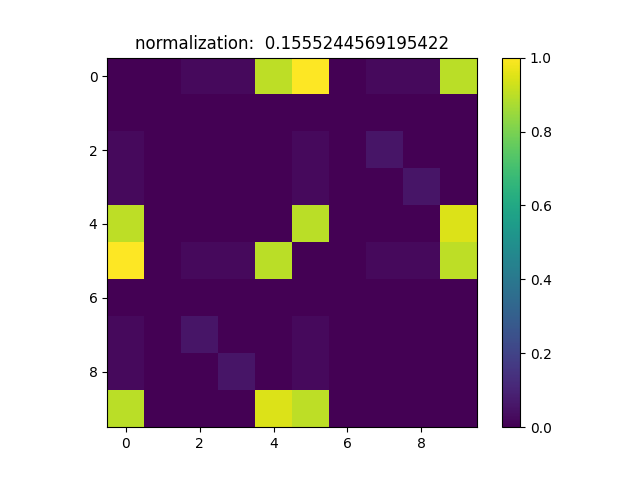}} \quad   
\subfloat[Groundstate in natural orbitals]
   {\includegraphics[width=0.45\textwidth]{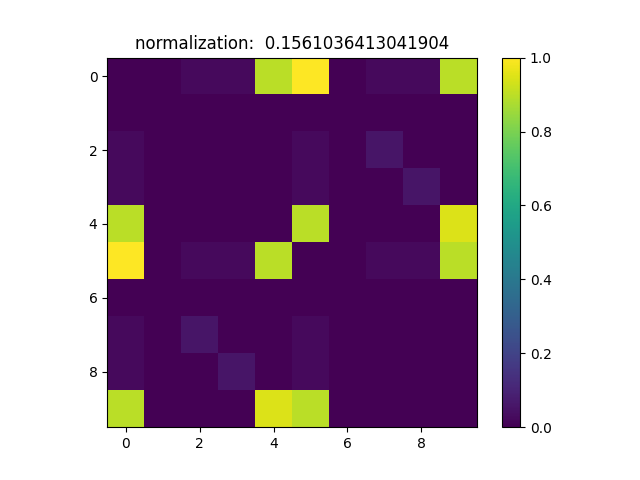}} \\
\caption{Quantum mutual information for $LiH$ molecule.}
\label{fig:LiH}
\end{figure*}

\begin{figure*}[!htb]
\centering
\subfloat[VQE state in HF canonical orbitals]
   {\includegraphics[width=0.45\textwidth]{grafici/supplementary/HF/VQE in initial basis.png}} \quad
\subfloat[WAHTOR state in WAHTOR-optimized orbitals]
   {\includegraphics[width=0.45\textwidth]{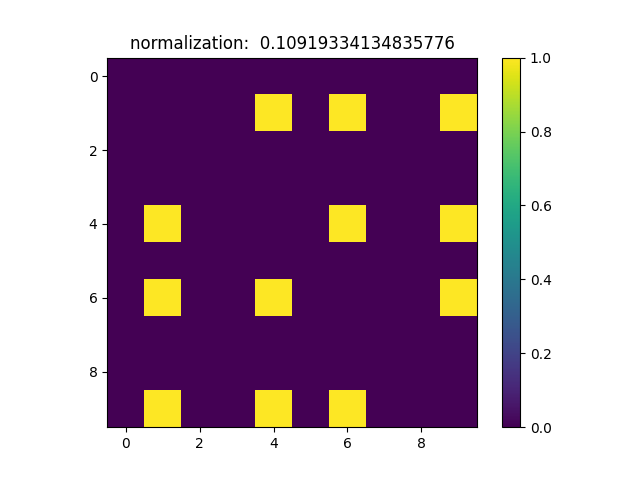}} \\
\subfloat[Groundstate in HF canonical orbitals]
   {\includegraphics[width=0.45\textwidth]{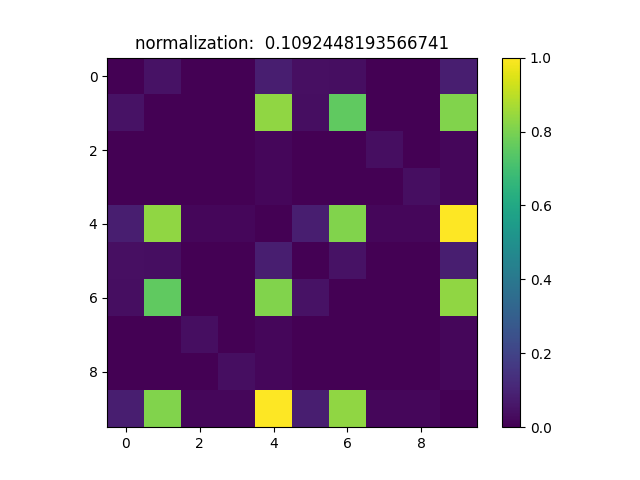}} \quad
\subfloat[Groundstate in WAHTOR-optimized orbitals]
   {\includegraphics[width=0.45\textwidth]{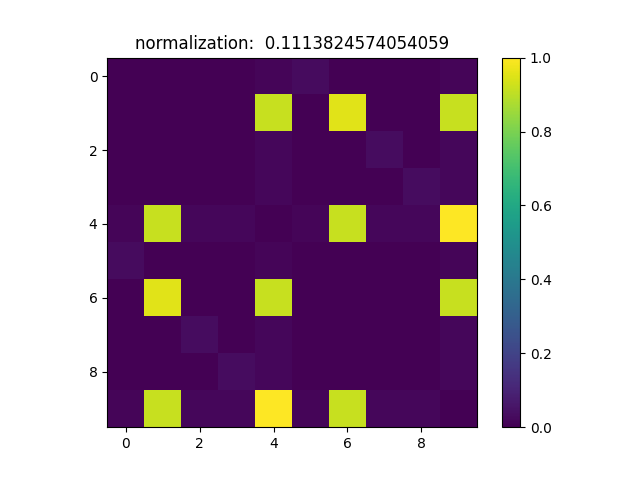}} \quad   
\subfloat[Groundstate in natural orbitals]
   {\includegraphics[width=0.45\textwidth]{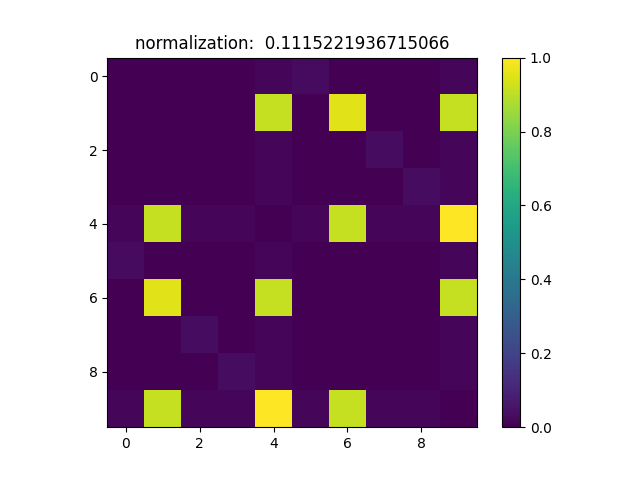}} \\
\caption{Quantum mutual information for $HF$ molecule.}
\label{fig:HF}
\end{figure*} 

\begin{figure*}[!htb]
\centering
\subfloat[VQE state in HF canonical orbitals]
   {\includegraphics[width=0.45\textwidth]{grafici/supplementary/BeH2/1/VQE in initial basis.png}} \quad
\subfloat[WAHTOR state in WAHTOR-optimized orbitals]
   {\includegraphics[width=0.45\textwidth]{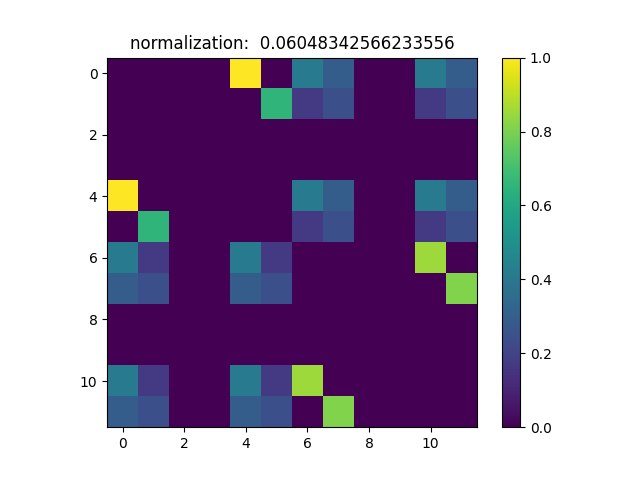}} \\
\subfloat[Groundstate in HF canonical orbitals]
   {\includegraphics[width=0.45\textwidth]{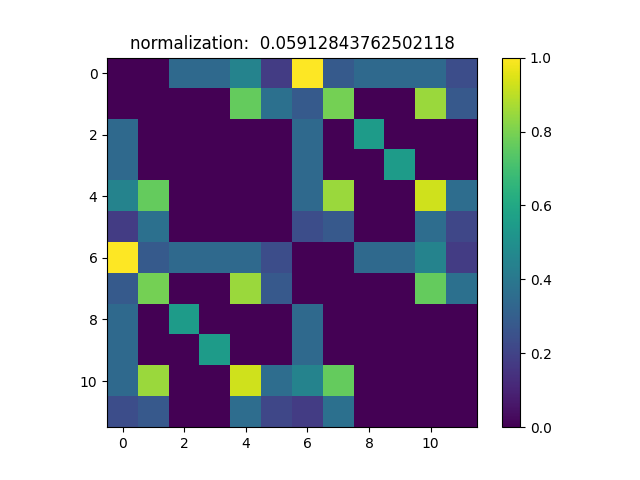}} \quad
\subfloat[Groundstate in WAHTOR-optimized orbitals]
   {\includegraphics[width=0.45\textwidth]{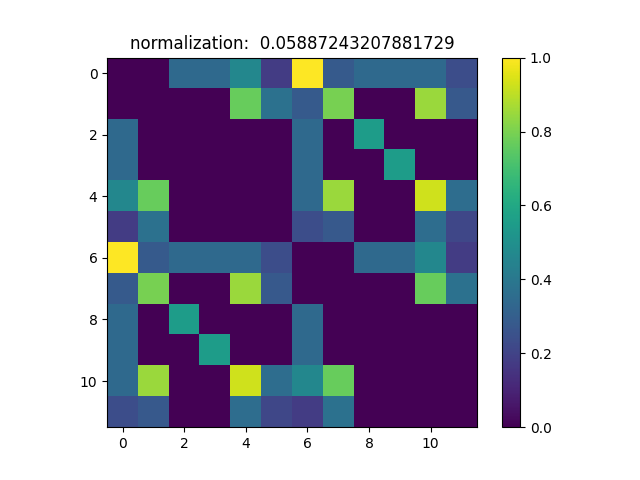}} \quad   
\subfloat[Groundstate in natural orbitals]
   {\includegraphics[width=0.45\textwidth]{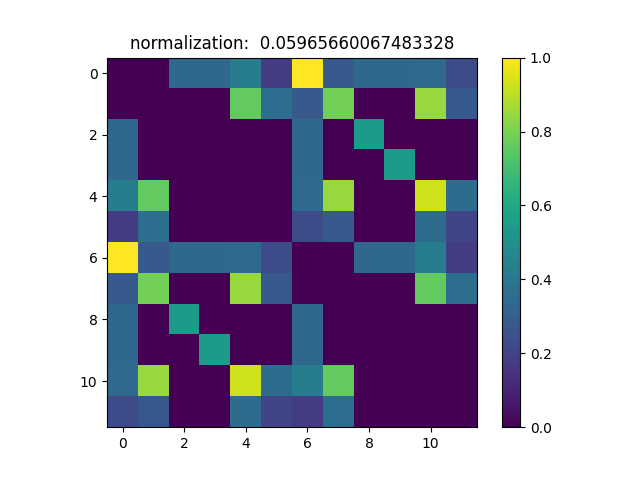}} \\
\caption{Quantum mutual information for $BeH_2$ molecule (case 1).}
\label{fig:BeH2}
\end{figure*} 

\begin{figure*}[!htb]
\centering
\subfloat[VQE state in HF canonical orbitals]
   {\includegraphics[width=0.45\textwidth]{grafici/supplementary/BeH2/2/VQE in initial basis.png}} \quad
\subfloat[WAHTOR state in WAHTOR-optimized orbitals]
   {\includegraphics[width=0.45\textwidth]{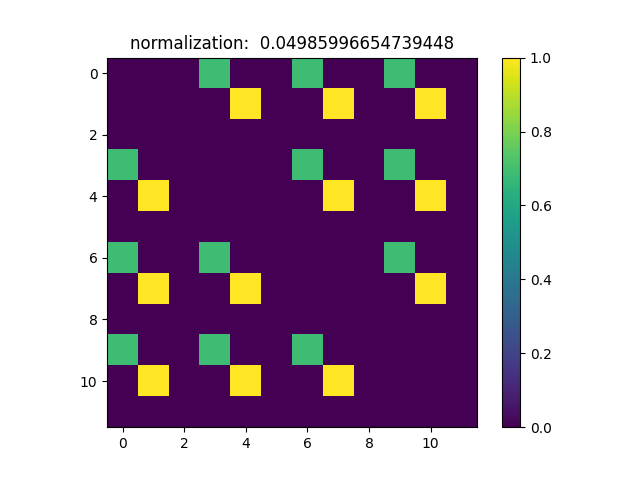}} \\
\subfloat[Groundstate in HF canonical orbitals]
   {\includegraphics[width=0.45\textwidth]{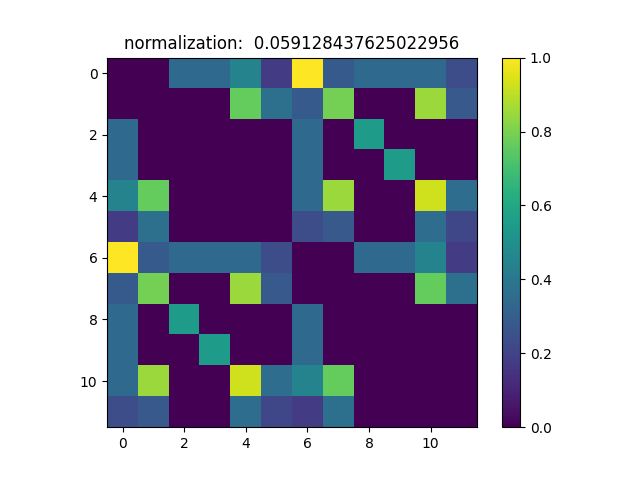}} \quad
\subfloat[Groundstate in WAHTOR-optimized orbitals]
   {\includegraphics[width=0.45\textwidth]{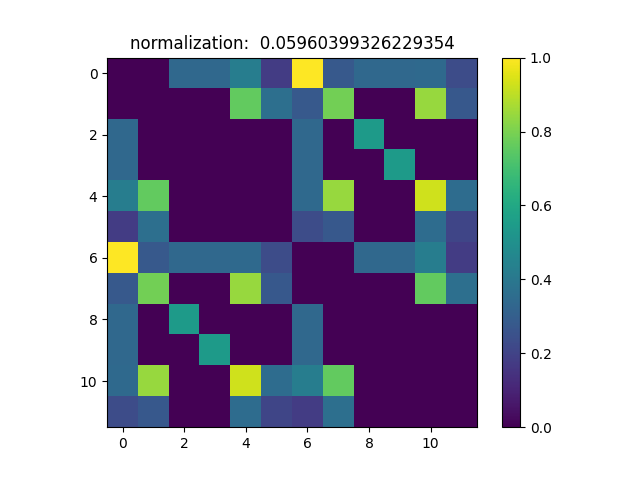}} \quad   
\subfloat[Groundstate in natural orbitals]
   {\includegraphics[width=0.45\textwidth]{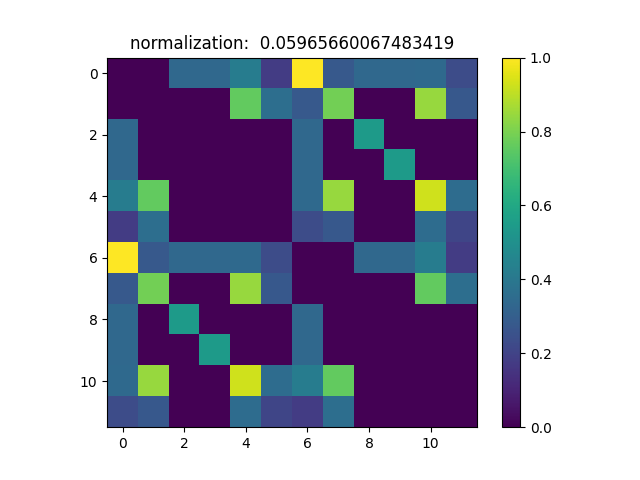}} \\
\caption{Quantum mutual information for $BeH_2$ molecule (case 2).}
\label{fig:BeH2}
\end{figure*} 

\begin{figure*}[!htb]
\centering
\subfloat[VQE state in HF canonical orbitals]
   {\includegraphics[width=0.45\textwidth]{grafici/supplementary/BeH2/3/VQE in initial basis.png}} \quad
\subfloat[WAHTOR state in WAHTOR-optimized orbitals]
   {\includegraphics[width=0.45\textwidth]{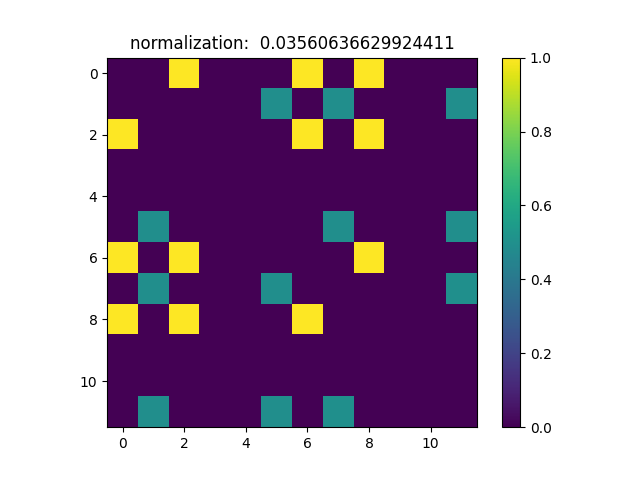}} \\
\subfloat[Groundstate in HF canonical orbitals]
   {\includegraphics[width=0.45\textwidth]{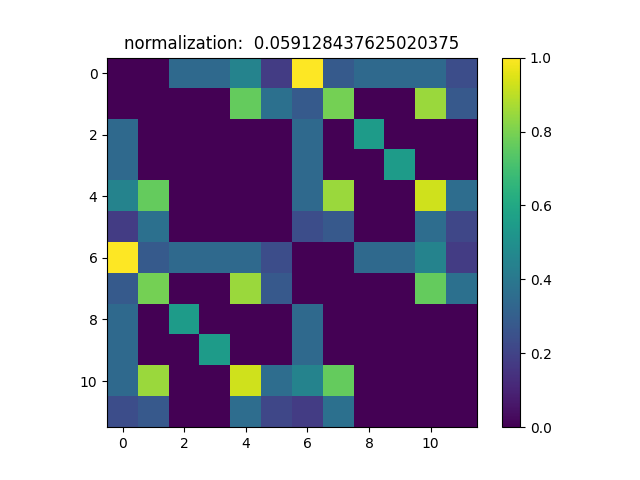}} \quad
\subfloat[Groundstate in WAHTOR-optimized orbitals]
   {\includegraphics[width=0.45\textwidth]{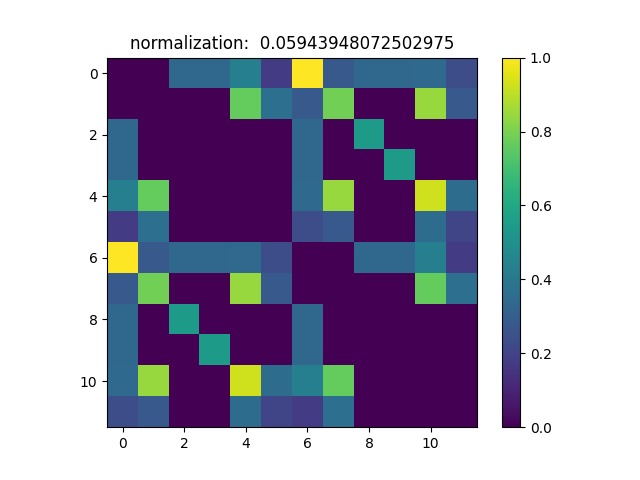}} \quad   
\subfloat[Groundstate in natural orbitals]
   {\includegraphics[width=0.45\textwidth]{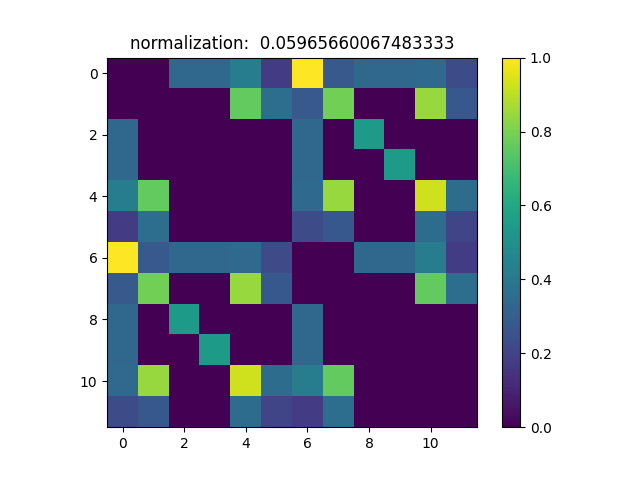}} \\
\caption{Quantum mutual information for $BeH_2$ molecule (case 3).}
\label{fig:BeH2}
\end{figure*} 

\begin{figure*}[!htb]
\centering
\subfloat[VQE state in HF canonical orbitals]
   {\includegraphics[width=0.45\textwidth]{grafici/supplementary/H2S/VQE in initial basis.png}} \quad
\subfloat[WAHTOR state in WAHTOR-optimized orbitals]
   {\includegraphics[width=0.45\textwidth]{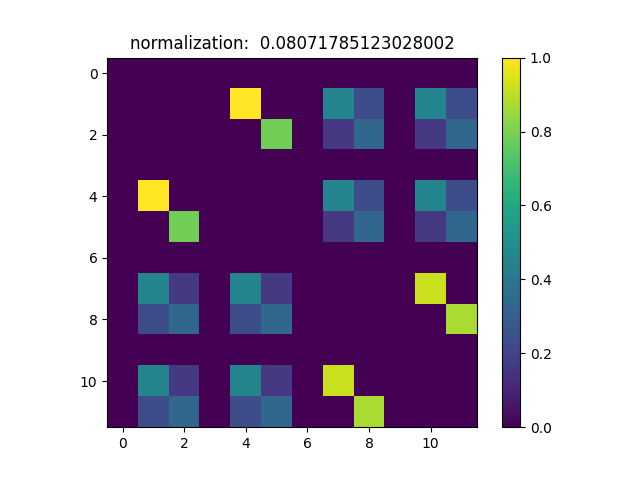}} \\
\subfloat[Groundstate in HF canonical orbitals]
   {\includegraphics[width=0.45\textwidth]{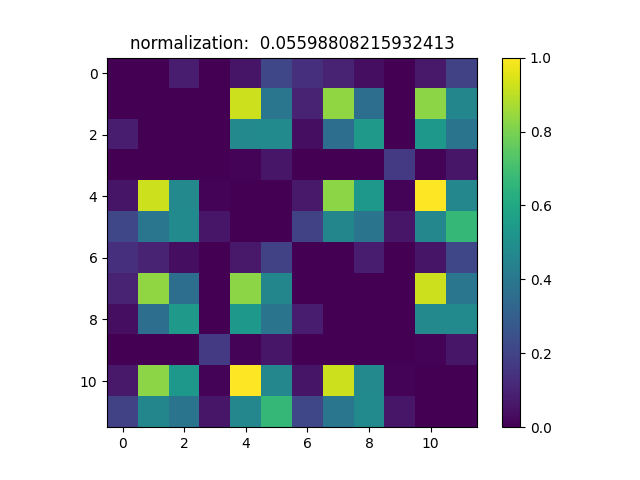}} \quad
\subfloat[Groundstate in WAHTOR-optimized orbitals]
   {\includegraphics[width=0.45\textwidth]{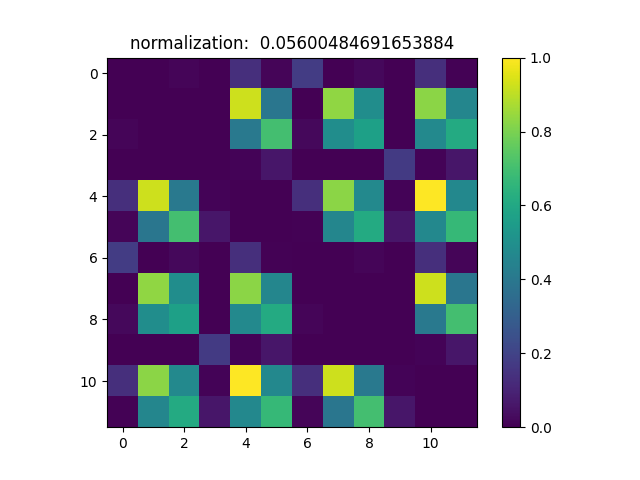}} \quad   
\subfloat[Groundstate in natural orbitals]
   {\includegraphics[width=0.45\textwidth]{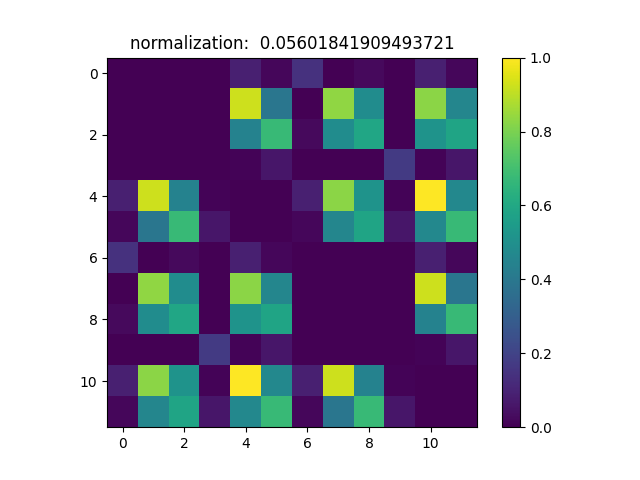}} \\
\caption{Quantum mutual information for $H_2S$ molecule.}
\label{fig:H2S}
\end{figure*} 

\begin{figure*}[!htb]
\centering
\subfloat[VQE state in HF canonical orbitals]
   {\includegraphics[width=0.45\textwidth]{grafici/supplementary/NH3/VQE in initial basis.png}} \quad
\subfloat[WAHTOR state in WAHTOR-optimized orbitals]
   {\includegraphics[width=0.45\textwidth]{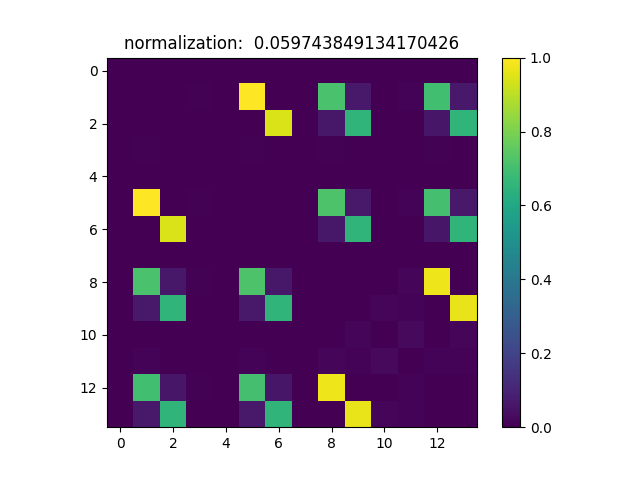}} \\
\subfloat[Groundstate in HF canonical orbitals]
   {\includegraphics[width=0.45\textwidth]{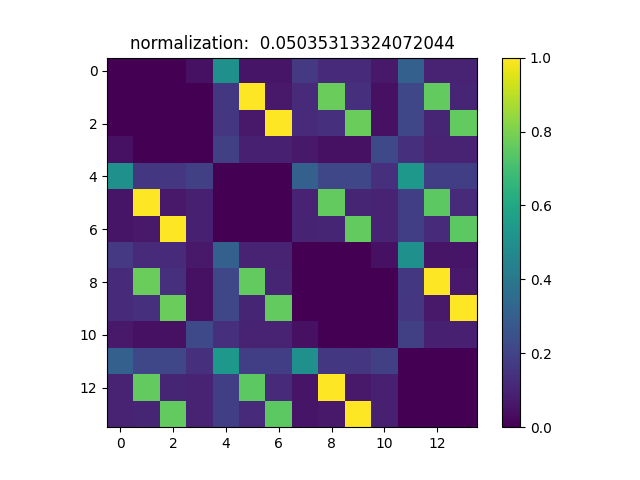}} \quad
\subfloat[Groundstate in WAHTOR-optimized orbitals]
   {\includegraphics[width=0.45\textwidth]{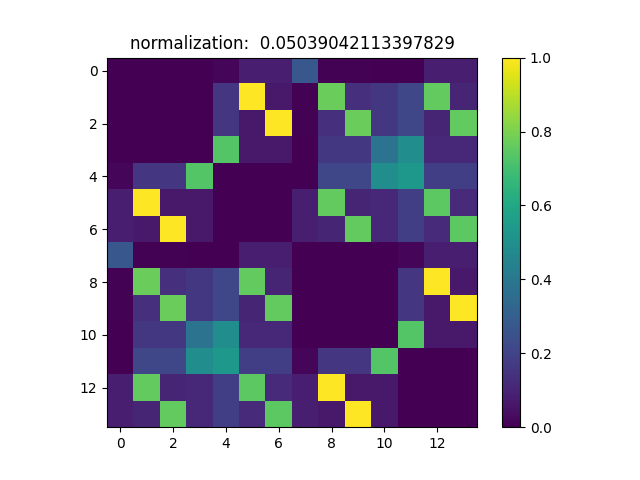}} \quad   
\subfloat[Groundstate in natural orbitals]
   {\includegraphics[width=0.45\textwidth]{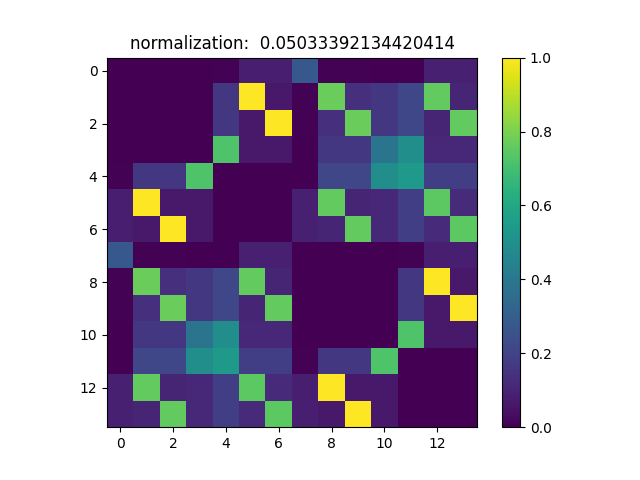}} \\
\caption{Quantum mutual information for $NH_3$ molecule.}
\label{fig:NH3}
\end{figure*} 

\end{document}
